# Supplementary material for: OVRseen: Auditing Network Traffic and Privacy Policies in Oculus VR
Source: arXiv:2106.05407 source file (2021-11-19)
Supplement: Supplementary file 1 [file additional.tex]

\subsection{Data Minimization}
We evaluate whether the transmission of data is necessary to the functionality of an Oculus App. For that purpose, we sample a few apps based on criteria such as if they were chatty. We also randomly sample a few apps to do the following:
\begin{itemize}
    \item Offline mode: We block all network traffic to see if they are still functional. 
    \item No platform mode: We block all network traffic going to Facebook.
    \item No X system apps: We block all network traffic initiated by certain system apps. We report which system apps are important to the functionality of apps.
    \item No network traffic from app: we block all network traffic initiated by the app itself.
\end{itemize}
